# Supplementary material for: Interface roughening in nonequilibrium phase-separated systems
Source: arXiv:2209.05096 ancillary file (2023-05-10)
Supplement: Supplementary file 1 [file qKPZ_supp.pdf]

# Supplementary material
# Interface roughening in nonequilibrium phase-separated systems


M. Besse,[1,2] G. Fausti,[1,3] M.E. Cates,[4] B. Delamotte,[2] and C. Nardini[1,2]

[1] *Service de Physique de l'Etat Condensé, CEA, CNRS Université Paris-Saclay, CEA-Saclay, 91191 Gif-sur-Yvette, France*
[2] *Sorbonne Université, CNRS, Laboratoire de Physique Théorique de la Matière Condensée, 75005 Paris, France*
[3] *Max Planck Institute for Dynamics and Self-Organization, 37077 Göttingen, Germany*
[4] *DAMTP, Centre for Mathematical Sciences, University of Cambridge, Wilberforce Road, Cambridge CB3 0WA, UK*



(Dated: March 5, 2023)


All through the Letter we use the following notation for the Fourier transform

$$\hat{h}(\mathbf{x},t) = \int \frac{d\mathbf{q}}{(2\pi)^d}\frac{d\omega}{2\pi} e^{-i\omega t + i\mathbf{q}\cdot\mathbf{x}} h(\mathbf{q},\omega) = \int_{\mathbf{q},\omega} e^{-i\omega t + i\mathbf{q}\cdot\mathbf{x}} h(\mathbf{q},\omega) \quad (1)$$

and analogously for other quantities.

### Appendix A: One-loop RG flow of |q|KPZ

We detail in this Appendix the one-loop RG for the $|\mathbf{q}|$KPZ equation.

#### 1. Perturbation theory

From the bare action (5), we define the propagator

$G_0(\mathbf{q},\omega) =$ 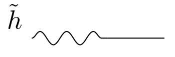 $= \dfrac{1}{-i\omega + \sigma|\mathbf{q}|\,\mathbf{q}^2}$, (A1)



and the vertices as

$V(\mathbf{q}_1,\mathbf{q}_2,\mathbf{q}_3) =$ 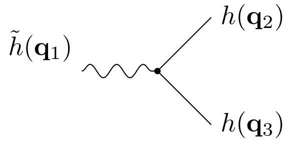 (A2)



$$= \frac{\lambda_1}{2}|\mathbf{q}_1|\,\mathbf{q}_2\cdot\mathbf{q}_3\;\delta(\mathbf{q}_1+\mathbf{q}_2+\mathbf{q}_3),$$

$N(\mathbf{q},\omega) =$ 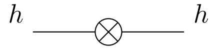 (A3)



$$= G_0(\mathbf{q},\omega)(-D|\mathbf{q}|)G_0(-\mathbf{q},-\omega)\,.$$

#### 2. Renormalization of the propagator

Renormalization of $\omega$ and $\sigma$ stems from the correction of diagram in Fig. (1a). For the renormalization of $\omega$, only terms proportional to $\omega$ at vanishing external momentum $\mathbf{p}$ matter. However, since the 3-leg vertex is proportional to the momentum carried on the $\tilde{h}$-leg, this contribution vanishes.

For the correction to $\sigma$, we have to extract from Fig. (1a) the terms proportional to $|\mathbf{p}|^3$ at vanishing external frequencies. This writes

$$I = 8\int_{\mathbf{q},\omega} V(\mathbf{p},\mathbf{q},-\mathbf{p}-\mathbf{q})N(\mathbf{q},\omega)V(\mathbf{p}+\mathbf{q},-\mathbf{q},-\mathbf{p}) \left. G_0(\mathbf{p}+\mathbf{q},\nu+\omega)\right|_{\nu=0}. \quad \text{(A4)}$$

The integral over the internal frequency in $I$ is calculated with the residue theorem, choosing the pole in the upper-left plane $\omega = i\sigma|\mathbf{q}|^3$:

$$I = \frac{D\lambda_1^2}{\sigma^2}\int_{\mathbf{q}} \frac{|\mathbf{p}|\,\mathbf{q}\cdot(\mathbf{p}+\mathbf{q})|\mathbf{p}+\mathbf{q}|\,\mathbf{p}\cdot\mathbf{q}|\mathbf{q}|}{|\mathbf{q}|^3\left(|\mathbf{q}|^3+|\mathbf{p}+\mathbf{q}|^3\right)}\,. \quad \text{(A5)}$$

To extract the contribution to the renormalization of $\sigma$, a Taylor expansion in small $\mathbf{p}$ is performed up to terms of order $|\mathbf{p}|^3$

$$I = \frac{D\lambda_1^2}{\sigma^2}\left(\frac{1}{2}\int_{\mathbf{q}}\frac{|\mathbf{p}|\mathbf{p}\cdot\mathbf{q}}{\mathbf{q}^2} + \frac{1}{4}\int_{\mathbf{q}}\frac{|\mathbf{p}|(\mathbf{p}\cdot\mathbf{q})^2}{\mathbf{q}^4}\right). \quad \text{(A6)}$$

The first term disappears by parity; Wilson's regularization up to a cutoff $\Lambda$ then gives at $d_c = 2$

$$I = \sigma|\mathbf{p}|^3\frac{D\lambda_1^2}{8\sigma^3}K_2\Lambda^{d-2}, \quad \text{(A7)}$$

where $K_2$ is the geometric angular factor of the momentum integration defined below Eq. (6).

#### 3. Nonrenormalization of the nonlinearity to one loop

The renormalization of $\lambda_1$ is obtained from the two diagrams in Fig. (1c) and (1d), where the graph in Fig. (1d) amounts to two contributions corresponding to the symmetrization with respect to the two external $h$-legs. Their sum, at order 3 in the external momenta and after integration over frequencies, writes

$$I_c + I_d \;\propto\; \frac{D\lambda_1^3}{\sigma^3}(2A_c - 2A_d)|\mathbf{p}_1| \int_{\mathbf{q}}\frac{\mathbf{q}\cdot\mathbf{p_2}\;\mathbf{q}\cdot(\mathbf{p_1}+\mathbf{p_2})}{\mathbf{q}^4}$$

where $A_c$ – resp. $A_d$ – is the combinatoric factor of the diagram (1c) – resp. (1d). Since $A_c = A_d$, $\lambda_1$ does not renormalize.

### 4. Nonrenormalization of the noise

From the diagram of Fig. (1b), corrections to the bare noise vertex are at least proportional to $\mathbf{p}^2$ ($\mathbf{p}$ is the external momentum). This is due to the fact that the 3-leg interaction vertex is proportional to the momentum carried by its $\tilde{h}$-leg. Thus there is no correction to the noise vertex, which is nonanalytic and of order $\mathbf{p}$.

### 5. RG flow in the unrescaled variables

Given the previous graphical corrections, the RG flow for the unrescaled variables $\sigma, \lambda_1$ and $D$ reads

$$\Lambda \frac{\mathrm{d}\sigma}{\mathrm{d}\Lambda} = (z - 3 + \frac{1}{8}\frac{D\lambda_1^2}{\sigma^3}K_2)\sigma, \tag{A8}$$

$$\Lambda \frac{\mathrm{d}\lambda_1}{\mathrm{d}\Lambda} = (z - 3 + \chi)\lambda_1, \tag{A9}$$

$$\Lambda \frac{\mathrm{d}D}{\mathrm{d}\Lambda} = (z - 2\chi - d - 1)D\,. \tag{A10}$$

Logarithmic differentiation of $g = D\lambda_1^2/\sigma^3$ together with Eq. (A8–A10) gives Eq. (6).

## Appendix B: Self-consistency of the |q|KPZ equation to one loop

We show in this Appendix that, although the $|\mathbf{q}|$KPZ equation (4) contains the singular mobility $|\mathbf{q}|$, it is stable to one loop under Wilson RG. More precisely, this means that no term that is more relevant (in RG sense) than those already included in the $|\mathbf{q}|$KPZ equation can be generated by fluctuations to one loop. We show this by *i*) proving in Appendix B 1 that symmetries constrain the operators generated along the RG flow and *ii*) by showing in Appendix B 2 that any nonlinearity generated to one loop is in the form of Eq. (3) with $g$ analytic in its arguments.

### 1. Two Ward identities for |q|KPZ

The bare action is invariant under two time-dependent (also called time-gauged) shift-symmetries, which write in Fourier space $\tilde{h}'(\mathbf{q},t) = \tilde{h}(\mathbf{q},t) + c_0(t)\delta(\mathbf{q})$ and $h'(\mathbf{q},t) = h(\mathbf{q},t) + c_0(t)\delta(\mathbf{q})$, where $c_0$ is an arbitrary smooth real function. From these symmetries, two identities for the effective action $\Gamma$ are inferred in the limit of infinitesimal $c_0(t)$:

$$\int_{\mathbf{q},t}\left(\frac{\delta\Gamma}{\delta\tilde{h}(\mathbf{q},t)} - \partial_t h(\mathbf{q})\right)c_0(t)\delta(\mathbf{q}) = 0, \tag{B1}$$

$$\int_{\mathbf{q},t}\left(\frac{\delta\Gamma}{\delta h(\mathbf{q},t)} + \partial_t \tilde{h}(\mathbf{q})\right)c_0(t)\delta(\mathbf{q}) = 0\,. \tag{B2}$$

Functional derivatives of these identities yield two Ward identities for the $(m,n)$-point vertices, $m,n \geq 1$,

$$\Gamma^{(m,n)}(\omega_1, \mathbf{q}_1 = \mathbf{0}, ..., Q_m|Q_{m+1}, ...) = i\omega_1\delta_{m,1}\delta_{n,1} \tag{B3}$$
$$\Gamma^{(m,n)}(...|\omega_{m+1}, \mathbf{q}_{m+1} = \mathbf{0}, ..., Q_{n+m}) = -i\omega_{m+1}\delta_{m,1}\delta_{n,1}.$$

where $\Gamma^{(m,n)}$ is defined as the $m$-th derivative with respect to $\tilde{h}$ and the $n$-th derivative with respect to $h$, the conservation of the total frequency and momentum being intended.

These two identities imply that, apart from the term $\int \tilde{h}\partial_t h$ which is not renormalized, all $\Gamma^{(m,n)}$ vanish upon setting one of their momenta to $\mathbf{0}$. This is true in any diagrammatic correction in the RG flow generated from the bare action (5), to any loop-order.

### 2. Functional form of the nonlinearities in the perturbative RG-flow of |q|KPZ

We show here that the functional form of the nonlinearities which is assumed in Eq. (3) is stable under one-loop corrections, as long as Eq. (5) is taken as the initial action of the RG flow.

Let us assume that, at the RG-scale $\Lambda$, the only nonanalytic terms in the $\Gamma^{(m,n)}(P_1, ..., P_m|P_{m+1}, ..., P_{m+n})$ are those attached to the $\tilde{h}(P_i)$-legs and are of the form $|\mathbf{p}_i|$. Therefore in any one-loop correction to the $\Gamma^{(m,n)}$'s

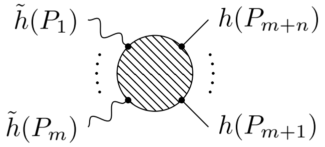


(B4)

the nonanalytic terms within the loop integral have the form $\left|\mathbf{q} + \sum_{i\in J}\mathbf{p}_i\right|$, $J$ being a subset of $\{1, ..., m+n\}$ and $\mathbf{q}$ the internal momentum. The momentum structure of the one-loop diagrams results from a Taylor expansion at small $\mathbf{p}_i$, hence is fully analytic in the external momenta $\mathbf{p}_i$. Therefore, at the RG scale $\Lambda - \mathrm{d}\Lambda$, the nonanalytic structure of the $\Gamma^{(m,n)}$ is the same as at scale $\Lambda$. Since the bare action satisfies to the assumption above about the momentum structure of the $\Gamma^{(m,n)}$, it stays true all along the flow.

As a consequence of appendix B 1 and of the argument above, nonlinearities have to be analytic in the momenta associated with the external $h$-legs. Moreover in any vertex of the RG flow (but $\int \tilde{h}\partial_t h$), each $\tilde{h}(Q)$ – resp. $h(Q)$ – is at least proportional to $|\mathbf{q}|$ – resp. to $\mathbf{q}$. The lowest order linear terms allowed by symmetries are thus $\partial_t h(\mathbf{q})$ and $|\mathbf{q}|\,\mathbf{q}^2 h(\mathbf{q})$, while the lowest order nonlinear term is $\lambda_1|\mathbf{q}|\,\mathcal{F}[|\nabla\hat{h}|^2](\mathbf{q})$, implying that the $|\mathbf{q}|$KPZ equation is stable under one-loop RG flow.

### Appendix C: Effective interface equations from AMB+

The linear description of capillary waves in active systems was obtained in [1] starting from AMB+, which is built itself upon a technique previously developed for passive fluids [2]. In this Appendix, we adapt this derivation to obtain the nonlinear terms.

We assume the absence of overhangs. On a rapid timescale, we expect diffusion to quasistatically relax $\phi(\mathbf{r},t)$ to a value that depends only on the distance to the interface. For small amplitude, long-wavelength perturbations, the vertical direction and the one normal to the interface are equivalent and we thus can assume that

$$\phi(\mathbf{r},t) = \varphi(y-\hat{h}(\mathbf{x},t)), \qquad \text{(C1)}$$

where $\varphi$ is the interfacial profile. For the derivation it is useful to introduce the pseudovariables $\psi$ and $g$ introduced in [3] for $\zeta=0$ and then generalized to AMB+ [4], which solve $K\partial^2\psi/\partial\phi^2 = (\zeta-2\lambda)\partial\psi/\partial\phi$ and $\partial g/\partial\psi = \partial f/\partial\phi \equiv \mu$, whence $\psi = K\left(\exp[(\zeta-2\lambda)\phi/K]-1\right)/(\zeta-2\lambda)$. In terms of them, the equilibrium conditions $\mu_1=\mu_2$ and $(\mu\psi-g)_1 = (\mu\psi-g)_2$ which select the binodals $\phi_{1,2}$ still hold [3, 4]. This change of variables is primarily a mathematical device for constructing the phase equilibria and simplify the calculations to obtain the equation for $h$; $\psi$ and $g$ have no direct physical significance beyond this. Let us also observe that while the Ansatz in Eq. (C1) is rigorously justified for deriving the linear (in $h$) terms at leading order in $|\mathbf{q}|$, a curvature-dependence in $\varphi$ can affect higher orders. Given that we are only interested in showing that $\lambda_1\neq 0$ emerges in the effective equation for the interface of AMB+ and not in finding the exact amplitude of these nonlinearities, we disregard a curvature-dependence in $\varphi$.

Following [1], we proceed by plugging Eq. (C1) into Eqs. (9–11) and inverting the Laplace operator (we assume Stratonovich's convention in the derivation). We multiply $\nabla^{-2}\partial_t\varphi$ by $\partial_y\psi$, integrate across the interface, Fourier transform along the $\mathbf{x}$-direction and expand in powers of $h$, to obtain Eq. (12), that we report here for convenience

$$\sum_{n=0}^{\infty}\int_{\mathbf{q}_1,\mathbf{x},\mathbf{x}_1}(-1)^n\frac{(\hat{h}(\mathbf{x})-\hat{h}(\mathbf{x}_1))^n}{2n!}|\mathbf{q}_1|^n\left\{A_n(\mathbf{q}_1)\partial_t\hat{h}(\mathbf{x})+\zeta D_n(\mathbf{q}_1)\nabla^2_{\mathbf{x}}\hat{h}\right\}e^{-i\mathbf{q}\cdot\mathbf{x}_1-i\mathbf{q}_1\cdot\mathbf{x}_1+i\mathbf{q}_1\cdot\mathbf{x}} = -\sigma_\lambda\mathbf{q}^2h_{\mathbf{q}}+\chi_{\mathbf{q}}, \qquad \text{(C2)}$$

where

$$\sigma_\lambda = K\int_y\psi'(y)\varphi'(y), \qquad \text{(C3)}$$

$$A_n(\mathbf{q}_1) = \int_{y_1,y_2}\mathrm{sgn}(y_1-y_2)^n\varphi'(y_1)\psi'(y_2)\frac{e^{-|\mathbf{q}_1||y_1-y_2|}}{|\mathbf{q}_1|},$$

$$D_n(\mathbf{q}_1) = \int_{y_1,y_2}\mathrm{sgn}(y_1-y_2)^{n+1}\varphi'^2(y_1)\psi'(y_2)e^{-|\mathbf{q}_1||y_1-y_2|}.$$

The noise $\chi_{\mathbf{q}}$ can be represented as a sum of Gaussian noises $\xi_n(\mathbf{q})$

$$\chi_{\mathbf{q}} = \sum_{n=0}^{\infty}\int_{\mathbf{q}_1}g^{(n)}_{\mathbf{q},\mathbf{q}_1}\xi_n(\mathbf{q}_1), \qquad \text{(C4)}$$

$$g^{(n)}_{\mathbf{q},\mathbf{q}_1} = \frac{1}{n!}\int_{\mathbf{x}}\hat{h}^n(\mathbf{x})e^{i(\mathbf{q}_1-\mathbf{q})\cdot\mathbf{x}},$$

where $\xi_n$ have zero average and correlations $\langle\xi_n(\mathbf{q}_1,t_1)\xi_m(\mathbf{q}_2,t_2)\rangle = C_{n,m}(\mathbf{q}_1)\delta(\mathbf{q}_1+\mathbf{q}_2)\delta(t_1-t_2)$, with

$$C_{n,m}(\mathbf{q}_1) = \frac{(2\pi)^dD}{|\mathbf{q}_1|}\int_{y_1,y_2}\psi'(y_1)\psi'(y_2)\partial^n_{y_1}\partial^m_{y_2}e^{-|\mathbf{q}_1||y_1-y_2|}$$

for $n+m$ even, while $C_{n,m}(\mathbf{q}_1)=0$ for $n+m$ odd. To leading order in $h$ and $\mathbf{q}$, Eq. (C2) reduces to Eq. (1), where the interfacial tension $\sigma$ is replaced by $2\sigma_{cw}/A$, with $\sigma_{\rm cw} = \sigma_\lambda + \frac{\zeta}{2}\int_{y_1,y_2}(y_1-y_2)\psi'(y_1)\varphi'^2(y_2)/|y_1-y_2|$ the capillary-waves interfacial tension and $A = \int_{y_1,y_2}\varphi'(y_1)\psi'(y_2)$ [1].

We now show how to obtain the terms in Eq. (C2) containing $\partial_t\hat{h}(\mathbf{x})$. The others can be obtained with a very similar procedure. We have to compute

$$\mathcal{F}_{\mathbf{x}\to\mathbf{q}}\left[\int_y\psi'(y-\hat{h}(\mathbf{x}))\nabla^{-2}\partial_t\phi(\mathbf{x},y)\right]. \qquad \text{(C5)}$$

By integration by parts, we obtain

$$\text{(C5)} = \int_{\mathbf{x},y}g_{\mathbf{q}}(\mathbf{x},y)\partial_t\phi(\mathbf{x},y) \qquad \text{(C6)}$$

where $g_{\mathbf{q}}(\mathbf{x},y)$ solves $\nabla^2g_{\mathbf{q}}(\mathbf{x},y) = e^{-i\mathbf{q}\cdot\mathbf{x}}\psi'(y-\hat{h}(\mathbf{x}))$. The function $g_{\mathbf{q}}$ can be expressed as [1]

$$g_{\mathbf{q}}(\mathbf{x},y) = -\frac{1}{2}\int_{\mathbf{q}_1,\mathbf{x}_1,y_1}\frac{e^{-|\mathbf{q}_1||y-y_1|}}{|\mathbf{q}_1|}e^{-i\mathbf{q}\cdot\mathbf{x}_1-i\mathbf{q}_1\cdot\mathbf{x}_1+i\mathbf{q}_1\cdot\mathbf{x}}\psi'(y_1-\hat{h}(\mathbf{x}_1)). \qquad \text{(C7)}$$

Using the Ansatz (C1), within Stratonovich's convention, we have $\partial_t\phi(\mathbf{x},y) = -\partial_t\hat{h}(\mathbf{x})\varphi'(y-\hat{h}(\mathbf{x}))$. Moreover, we perform the change of variables $y\to y-\hat{h}(\mathbf{x})$, $y_1\to$

$y_1 - \hat{h}(\mathbf{x})$ and Taylor expand for small $\hat{h}(\mathbf{x}) - \hat{h}(\mathbf{x}_1)$. We obtain:

$$(\text{C5}) = \frac{1}{2}\sum_{n=0}^{\infty}\int_{\mathbf{q}_1,\mathbf{x},y,\mathbf{x}_1,y_1} e^{-i\mathbf{q}\cdot\mathbf{x}_1 - i\mathbf{q}_1\cdot\mathbf{x}_1 + i\mathbf{q}_1\cdot\mathbf{x}}\frac{\tilde{A}_n(\mathbf{q}_1)}{|\mathbf{q}_1|} \frac{(\hat{h}(\mathbf{x}) - \hat{h}(\mathbf{x}_1))^n}{n!}\partial_t\hat{h}(\mathbf{x}), \quad (\text{C8})$$

$$\tilde{A}_n(\mathbf{q}_1) = \int_{y,y_1}\varphi'(y)\psi^{(1+n)}(y_1)e^{-|\mathbf{q}_1\|y-y_1|}\,. \quad (\text{C9})$$

Finally, integrating $\tilde{A}_n(\mathbf{q}_1)$ by parts $n$ times over $y_1$ and observing that some of the terms vanish by integrating over $\mathbf{q}_1$, gives the desired result.

### 1. Effective interface equation in the Ito convention

We now transform Eq. (C2) to a stochastic equation within the Ito's convention. We begin by rewriting Eq. (C2) as

$$\partial_t h_{\mathbf{q}} + \int_{\mathbf{q}_1}\mathcal{L}^{-1}_{\mathbf{q},\mathbf{q}_1}\left[\zeta\mathcal{M}_{\mathbf{q}_1} + \sigma_\lambda \mathbf{q}_1^2 h_{\mathbf{q}_1}\right] = \sum_{n=0}^{\infty}\int_{\mathbf{q}_1,\mathbf{q}_2}\mathcal{L}^{-1}_{\mathbf{q},\mathbf{q}_1} g^{(n)}_{\mathbf{q}_1,\mathbf{q}_2}\xi_n(\mathbf{q}_2), \quad (\text{C10})$$

where

$$\mathcal{L}_{\mathbf{q},\mathbf{q}_1} = \sum_{n=0}^{\infty}\int_{\mathbf{q}_2,\mathbf{x},\mathbf{x}_1}(-1)^n\frac{(\hat{h}(\mathbf{x}) - \hat{h}(\mathbf{x}_1))^n}{2n!} |\mathbf{q}_2|^n A_n(\mathbf{q}_2)e^{-i\mathbf{q}\cdot\mathbf{x}_1 - i\mathbf{q}_2\cdot\mathbf{x}_1 + i\mathbf{q}_2\cdot\mathbf{x} + i\mathbf{q}_1\cdot\mathbf{x}}, \quad (\text{C11})$$

and

$$\mathcal{M}_{\mathbf{q}_1} = \sum_{n=0}^{\infty}\int_{\mathbf{q}_2,\mathbf{x},\mathbf{x}_1}(-1)^n\frac{(\hat{h}(\mathbf{x}) - \hat{h}(\mathbf{x}_1))^n}{2n!} |\mathbf{q}_2|^n D_n(\mathbf{q}_2)\nabla^2_{\mathbf{x}}\hat{h}\, e^{-i\mathbf{q}_1\cdot\mathbf{x}_1 - i\mathbf{q}_2\cdot\mathbf{x}_1 + i\mathbf{q}_2\cdot\mathbf{x}}\,. \quad (\text{C12})$$

The operator $\mathcal{L}^{-1}$ is defined as the inverse operator of $\mathcal{L}$ by

$$\int_{\mathbf{q}_1}\mathcal{L}^{-1}_{\mathbf{q},\mathbf{q}_1}\mathcal{L}_{\mathbf{q}_1,\mathbf{p}} = \delta(\mathbf{q}_1 - \mathbf{p})\,. \quad (\text{C13})$$

Following the standard procedure [5, 6] we obtain the effective equation for the interface of AMB+ within the Ito's convention

$$\partial_t h_{\mathbf{q}} + \int_{\mathbf{q}_1}\mathcal{L}^{-1}_{\mathbf{q},\mathbf{q}_1}\left[\zeta\mathcal{M}_{\mathbf{q}_1} + \sigma_\lambda \mathbf{q}_1^2 h_{\mathbf{q}_1}\right] = \sum_{n=0}^{\infty}\int_{\mathbf{q}_1,\mathbf{q}_2}\mathcal{L}^{-1}_{\mathbf{q},\mathbf{q}_1} g^{(n)}_{\mathbf{q}_1,\mathbf{q}_2}\xi_n(\mathbf{q}_2) + \mathcal{I}_{S\to I}(\mathbf{q}), \quad (\text{C14})$$

where

$$\mathcal{I}_{S\to I}(\mathbf{q}) = \frac{1}{2}\sum_{n,m=0}^{\infty}\int_{\mathbf{q}_1,\ldots,\mathbf{q}_5,\mathbf{x}}\frac{\delta}{\delta\hat{h}(\mathbf{x})}\left[\mathcal{L}^{-1}_{\mathbf{q},\mathbf{q}_1}g^{(n)}_{\mathbf{q}_1,\mathbf{q}_2}\right]e^{i\mathbf{q}_3\cdot\mathbf{x}} \mathcal{L}^{-1}_{\mathbf{q}_3,\mathbf{q}_4}g^{(m)}_{\mathbf{q}_4,\mathbf{q}_5}C_{n,m}(\mathbf{q}_2)\delta(\mathbf{q}_2 + \mathbf{q}_5)\,. \quad (\text{C15})$$

### 2. Irrelevance of singular nonlinearities

Eq. (C14) and (C15) contain nonlinearities in the form of Eq. (3) with $g$ singular. We show here that they are all irrelevant close to $d = 2$ from RG viewpoint.

We denote by $\Lambda$ the momentum scale. It is straightforward to see that all nonlinearities in Eq. (C14) but those in the noise term and in $\mathcal{I}_{S\to I}$ are irrelevant by RG dimensional analysis. Furthermore, the leading order noise is $\xi_0$, which is of order $\mathcal{O}(\Lambda^{-1/2})$. Because $\hat{h}$ is dimensionless at the upper critical dimension ($d = 2$) and all covariances $\langle\xi_n(\mathbf{q}_1, t_1)\xi_m(\mathbf{q}_2, t_2)\rangle$ are at least of order $\mathcal{O}(\Lambda^0)$ unless $n = m = 0$, it follows that all $\xi_n$ with $n \geq 1$ are irrelevant close to $d = 2$. The same result can be obtained in a more direct way observing that, within Ito's convention, the noise variance $\chi_{\mathbf{q}}$ can be written as

$$\langle\chi_{\mathbf{q}_1}(t_1)\chi_{\mathbf{q}_2}(t_2)\rangle = \sum_{n=0}^{\infty}\int_{\mathbf{x}_1,\mathbf{x}_2,\mathbf{q}}(-1)^n\frac{(\hat{h}(\mathbf{x}_1) - \hat{h}(\mathbf{x}_2))^n}{n!} \times|\mathbf{q}|^n B_n(\mathbf{q})e^{-i(-\mathbf{q}+\mathbf{q}_1)\cdot\mathbf{x}_1 - i(\mathbf{q}+\mathbf{q}_2)\cdot\mathbf{x}_2}\delta(t_1 - t_2)\,,$$

where

$$B_n(\mathbf{q}) = D\int_{y_1,y_2}\text{sgn}(y_1 - y_2)^n\psi'(y_1)\psi'(y_2)\frac{e^{-|\mathbf{q}\|y_1-y_2|}}{|\mathbf{q}|}\,.$$

We are now left with showing that the terms in $\mathcal{I}_{S\to I}$ are also irrelevant. To show this, it is useful to notice that the leading order in $\mathcal{L}$ is $\Lambda^{-d-1}$ so that, from Eq. (C13), the leading order in $\mathcal{L}^{-1}$ is $\Lambda^{-d+1}$. We will furthermore use the scalings $\delta/\delta\hat{h}(\mathbf{x}) \sim \Lambda^d\hat{h}^{-1}$, $g^{(n)} \sim \Lambda^{-d}\hat{h}^n$, $\hat{h} \sim \Lambda^{(d-2)/2}$ and $t^{-1} \sim \Lambda^3$.

We first restrict to $n \geq 1$. In this case, $C_{n,m}$ scales at least as $\Lambda^0$; along with the observations above, it allows to show that nonlinearities with $n \geq 1$ are irrelevant close to $d = 2$. Finally, when $n = 0$, the functional derivative must act on $\mathcal{L}^{-1}$. Performing the functional derivative of Eq. (C13) with respect to $\hat{h}(\mathbf{x})$ and using (C11), it can be shown that the contribution at $\mathcal{O}(\hat{h}^{m-1})$ of $\delta\mathcal{L}^{-1}_{\mathbf{q},\mathbf{p}}/\delta\hat{h}(\mathbf{x})$ scales at least as $\Lambda^{m+1}\hat{h}^{m-1}$ with $m \geq 1$. This allows to infer that also the nonlinearities with $n = 0$ are irrelevant close to $d = 2$ and concludes our argument.

### 3. Generation of $\lambda_1$ from fluctuations

The derivation of the interface equation from AMB+ gives $\lambda_1 = 0$ at bare level. We have furthermore shown that all nonlinearities are irrelevant from dimensional analysis. Here we finally argue that $\lambda_1 \neq 0$ is generated upon fluctuations. Given the implicit form of Eq. (C14) we do not perform a full one-loop RG analysis and restrict to find a one-loop diagram that generates $\lambda_1 \neq 0$. As discussed in the main text, we thus expect that interfaces of active phase-separated systems are described by the $|\mathbf{q}|$KPZ equation.

It is first convenient to rewrite Eq. (C14) as

$$\int_{\mathbf{q}_1} \mathcal{L}_{\mathbf{q},\mathbf{q}_1} \partial_t h_{\mathbf{q}_1} + \sigma_\lambda \mathbf{q}^2 h_{\mathbf{q}} + \zeta \mathcal{M}_{\mathbf{q}} \qquad \text{(C16)}$$
$$= \sum_{n=0}^{\infty} \int_{\mathbf{q}_1} g^{(n)}_{\mathbf{q},\mathbf{q}_1} \xi_n(\mathbf{q}_1) + \int_{\mathbf{q}_1} \mathcal{L}_{\mathbf{q},\mathbf{q}_1} \mathcal{I}_{S\to I}(\mathbf{q}_1)\,.$$

To show that $\lambda_1$ is generated along the RG flow we need to take into account nonlinearities of order $\mathcal{O}(h^3)$. Indeed, [7] suggests that quadratic nonlinearities do not produce, upon renormalization to one-loop, another quadratic nonlinearity. Quadratic nonlinearities can instead be produced contracting a cubic with a quadratic nonlinearities.

For instance, to one loop, taking into account the nonlinearity of order $\mathcal{O}(h\partial_t h)$ and $\mathcal{O}(h^2\partial_t h)$ in Eq. (C16), the diagrams that can generate corrections to $\lambda_1$ are those in Fig. 1. We have checked that the diagram in Fig. 1a gives corrections proportional to $|\mathbf{q}|^3 \mathcal{F}[(\nabla_{\mathbf{x}} h)^2]$ and to $|\mathbf{q}| \int_{Q+Q_2+Q_3=0} \mathbf{q}\cdot\mathbf{q}_2\ \mathbf{q}\cdot\mathbf{q}_3 h(Q_2)h(Q_3)$. Instead, the diagram in Fig. 1b yields a correction proportional to $|\mathbf{q}| \mathcal{F}[(\nabla_{\mathbf{x}} h)^2]$, implying that $\lambda_1 \neq 0$ is indeed generated.

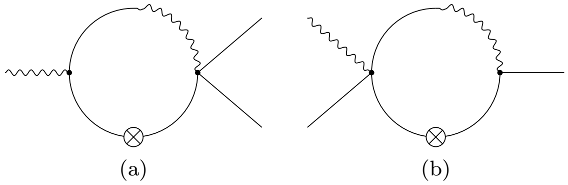

Figure 1. Two graphical corrections to the 3-leg vertex.

It should be finally observed that in the specific case of equilibrium Model B, the same argument for generating $\lambda_1$ does not apply, consistently. In this case, indeed, $\zeta = 0$ ; hence $\psi = \varphi$ and $A_{2n+1}(\mathbf{q}) = 0$. Using also that $C_{n,m} = 0$ for $n+m$ odd, it follows that Eq. (C16) is invariant under the symmetry $h \to -h$ and thus $\lambda_1$ cannot be generated by fluctuations.


[1] G. Fausti, E. Tjhung, M. Cates, and C. Nardini, Phys. Rev. Lett. **127**, 068001 (2021).

[2] A. J. Bray, A. Cavagna, and R. D. Travasso, Phys. Rev. E **65**, 016104 (2001).

[3] A. P. Solon, J. Stenhammar, M. E. Cates, Y. Kafri, and J. Tailleur, Phys. Rev. E **97**, 020602 (2018).

[4] E. Tjhung, C. Nardini, and M. E. Cates, Phys. Rev. X **8**, 031080 (2018).

[5] C. W. Gardiner *et al.*, *Handbook of stochastic methods*, Vol. 3 (Springer Berlin, 1985).

[6] M. E. Cates, É. Fodor, T. Markovich, C. Nardini, and E. Tjhung, Entropy **24**, 254 (2022).

[7] H. Janssen, Phys. Rev. Lett. **78**, 1082 (1997).
